# Supplementary material for: Dark Energy Survey Year 3 results: Magnification modeling and impact on cosmological constraints from galaxy clustering and galaxy-galaxy lensing
Source: arXiv:2209.09782 source file (2023-05-26)
Supplement: Supplementary file 1 [file appendix_mag_formalism.tex]

\section{Magnification Formalism}

 Magnification produces an increase in the solid angle occupied by the observed image $d \Omega^\text{obs}$ with respect to the one we would observe without gravitational lensing $d \Omega^\text{int}$ and it can be defined as:
\begin{equation}\label{eq:magnification}
 \mu = \frac{d \Omega^\text{obs}}{d \Omega^\text{int}}
\end{equation}

Then, magnification produces a "stretch" of the image, making the whole field larger and increasing the size of the galaxies as well. On the other hand, from Liouville's theorem it can be derived that the surface brightness $I$, which is the flux $F$ per unit solid angle of the image $d\Omega$, is conserved in all gravitational lensing processes where the light is neither created nor destroyed, just redistributed. Therefore, the total flux of a magnified galaxy, which is the integral of the surface brightness over the corresponding area, will be larger than it would have been without magnification. Therefore, due to surface brightness conservation and together with Eq.~(\ref{eq:magnification}), the ratio of the image flux $F^\text{obs}$ and source flux $F^\text{int}$ is also the magnification:
\begin{equation}\label{eq:surface_brightness}
    I = \frac{F^\text{int}}{d \Omega^\text{int}} = \frac{F^\text{obs}}{d \Omega^\text{obs}} \quad \Rightarrow \quad \mu = \frac{d \Omega^\text{obs}}{d \Omega^\text{int}} = \frac{F^\text{obs}}{F^\text{int}}.
\end{equation}
